# Supplementary material for: Dispider: Enabling Video LLMs with Active Real-Time Interaction via Disentangled Perception, Decision, and Reaction
Source: arXiv:2501.03218 source file (2025-01-06)
Supplement: Supplementary file 1 [file suppl.tex]

\clearpage
\setcounter{page}{1}
\maketitlesupplementary
